# Supplementary material for: Distributed Constrained Online Learning
Source: arXiv:1903.06310 source file (2019-03-15)
Supplement: Supplementary file 1 [file appendix_old.tex]

%!TEX root = root.tex
\appendix
\section{Appendices}
\subsection{Proof of Theorem \ref{theo_main}}\label{ap_main}
%

In the generic case, by virtue of Assumption \ref{assumption_bound} we have %
\begin{equation}
\int_0^Tf_0(t,\bbx(t)) - f_0(t,\bbx^*)dt \geq -\int_0^T Kdt = -KT.
\end{equation}
%
Using this bound and selecting $\tilde{\bm{\mu}}=0$ \eqref{eqn_key_lemma} reduces to
%
\begin{equation}\label{eqn_key_eq_appendix}
\begin{split}
      \sum_{i=1}^N \int_0^T\left[\tilde{\bm{\lambda}}_i^\top f_i(t,\bbx_i(t))-\bm{\lambda}_i^\top(t)f_i(t,\tilde{\bbx})\right] \,dt\\
      -\sum_{i=1}^N \sum_{j\in \ccalN_i} \int_0^T\mu_{ij}(t)\left(\left\|\tilde{\bbx}_i-\tilde{\bbx}_j\right\|^2 -\gamma\right) \, dt  \\ 
      \leq \frac{1}{\varepsilon}V_{\tilde{\bbx},\tilde{\bm{\lambda}},\tilde{\bm{\mu}}}(\bbx_d(0),{\bm{\lambda}}_d(0),\bm{\mu}(0)) + KT
\end{split}
    \end{equation}
%

Observe that by selecting $\tilde{\bbx} =\bbx^*$, the solution of the centralized problem \eqref{eqn_optimization_problem},  we have that $f_i(t,\tilde{\bbx}) <0$. Moreover, using the fact that the Lagrange Multipliers $\bm{\lambda}_i(t)$ are in the positive orthant (c.f. \eqref{eqn_gradient_ascent_lambda}) the product $-\bm{\lambda}_i^\top(t)f_i(t,\tilde{\bbx})$ is always positive. Likewise, the product $\mu_ij(t)\left(\gamma-\left\|\bbx_i^*-\bbx_j^*\right\|^2\right)\geq 0.$ Denote by  $\left[\cdot \right]^+$ the projection over the positive orthant. Then, for a particular $i$ choose $\tilde{\bm{\lambda}}_i = \left[\ccalF_T^{ii} \right]^+$ and chose $\tilde{\bm{\lambda}}_j= \bm{0}$ for all $j\neq i$. Then, \eqref{eqn_key_eq_appendix} reduces to 
%
\begin{equation}
\begin{split}
      \left\| \left[\ccalF_T^{ii}\right]^+\right\|^2
      \leq \frac{1}{2}V_{\tilde{\bbx},\tilde{\bm{\lambda}},\tilde{\bm{\mu}}}(\bbx_d(0),{\bm{\lambda}}_d(0),\bm{\mu}(0)) + KT.
\end{split}
    \end{equation}
    %
    Hence it follows that the local fit is bounded by a function that is of the order of $O(\sqrt{T})$. The proof is then completed by using the Liptchitz continuity of the functions $f_i(t,\bbx)$ (c.f. Assumption \ref{assumption_convexity}) and the sublinear network disagreement (c.f. Proposition \ref{proposition_disagreement}), as it was done in the case with objective function independent of $\bbx$.
